# Supplementary material for: TileLink: Generating Efficient Compute-Communication Overlapping Kernels using Tile-Centric Primitives
Source: arXiv:2503.20313 source file (2025-04-03)
Supplement: Supplementary file 1 [file appendix.tex]

\section{Hello World}
%\subsection{Hello World}
